# Supplementary material for: Regularizing Black-box Models for Improved Interpretability
Source: arXiv:1902.06787 source file (2020-11-08)
Supplement: Supplementary file 1 [file theory.tex]

\subsection{Details on the Generalization of Local Linear Explanations}
\label{appendix:generalization}

Here, we provide a derivation of the bound \eqref{eq:fidelity-bound-in-probability-hoeffding} on the explanation fidelity.
First, we assume that local linear explanations, $\beta_x$, are obtained by solving the ordinary least squares regression problem (as given in Algorithm~\ref{alg:expo-fidelity-reg}):
\begin{equation}
    \beta_x = \left[X' X'^\top\right]^{-1} X' f(X'),
\end{equation}
where each column of $X'$ denotes a sample from the neighborhood $N_x$ and $f(X')$ is a column-vector of the corresponding function values.
The \emph{expected} fidelity of the explanation $\beta_x$ can be computed analytically:
\begin{equation}
    \label{eq:expected-residual-ordinary-regression}
    r(f, x) = \ep[N_x]{f(x')^2} - \ep[N_x]{f(x') x'}^\top \ep[N_x]{[x' x'^\top]}^{-1} \ep[N_x]{f(x') x'}
\end{equation}
where expectation $\ep[N_x]{\cdot}$ is taken with respect to $x'$ over the neighborhood $N_x$.
Note the equality in \eqref{eq:expected-residual-ordinary-regression} is the expected value of the squared residual between $f(x)$ and the optimal local linear explanation, which is upper-bounded by the variance of the model in the corresponding neighborhood:
\begin{equation}
    \label{eq:expected-residual-ordinary-regression-upper-bound}
    0 \leq r(f, x) \leq \ep[N_x]{f(x')^2} - \ep[N_x]{f(x')}^2 = \var[N_x]{f(x')}
\end{equation}
For instance, if $f(x)$ is $L$-Lipschitz and the neighborhood $N_x$ is defined a uniform distribution within a $\sigma$-ball centered at $x$, then the variance of $f(x)$ within the neighborhood can be further bounded by $4L^2\sigma^2$, hence $r(f, x) \leq 4L^2\sigma^2$.

For the explanations to generalize, we would like to make sure that the gap between the average fidelity on the training set and the expected fidelity is small with high probability.
More formally, the following inequality should hold:
\begin{equation}
    \label{eq:fidelity-bound-in-probability-generic}
    \prob{\ep{r(f, x)} - \frac{1}{n} \sum_{i=1}^n r(f, x_i) > \varepsilon} < \delta_n(\varepsilon)
\end{equation}
The following is a restatement of Proposition~\ref{prop:explanation-generalization} with a short proof.

\begin{proposition}
    Let the neighborhood sampling function $N_x$ be characterized by some parameter $\sigma$ (\eg, the effective radius of a neighborhood) and the variance of the trained model $f(x)$ across all such neighborhoods be bounded by some constant $C(\sigma) > 0$.
    Then, the following bound holds with at least $1 - \delta$ probability:
    \begin{equation*}
        \ep{r(f, x)} \leq \frac{1}{n} \sum_{i=1}^n r(f, x_i) + \sqrt{\frac{C^2(\sigma)\log\frac{1}{\delta}}{2n}}
    \end{equation*}
\end{proposition}
\begin{proof}
    By assumption, the variance of the model $f(x)$ is bounded in each local neighborhood specified by $N_x$.
    Then \eqref{eq:expected-residual-ordinary-regression} implies that each residual is bounded as $0 \leq r(f, x) \leq C(\sigma)$.
    Applying Hoeffding's inequality, we get:
    \begin{equation*}
        \label{eq:fidelity-bound-hoeffding}
        \prob{\ep{r(f, x)} - \frac{1}{n} \sum_{i=1}^n r(f, x_i) > \varepsilon} < \exp\left\{\frac{-2n\varepsilon^2}{C^2(\sigma)}\right\}
    \end{equation*}
    Inverting the inequality gives us the bound.
\end{proof}
